# Supplementary material for: Kafka Consumer Group Autoscaler
Source: arXiv:2206.11170 source file (2022-06-22)
Supplement: Supplementary file 1 [file modified_any_fit.tex]

\section{Modified Any Fit Algorithm}
